# Supplementary material for: Visualization of defect-induced interband proximity effect at the nanoscale
Source: arXiv:2505.06072 ancillary file (2025-07-07)
Supplement: Supplementary file 1 [file Interband_coupling_supplemental.pdf]

## Supplementary Materials

# Engineering Interband Coupling of a Two-band Superconductor by Topological Defects

Thomas Gozliniski,<sup>1,\*</sup> Qili Li,<sup>1,†</sup> Rolf Heid,<sup>2</sup> Oleg Kurnosikov,<sup>3</sup> Alexander Haas,<sup>1</sup>  
Ryohei Nemoto,<sup>4</sup> Toyo Kazu Yamada,<sup>4,5</sup> Jörg Schmalian,<sup>6,7</sup> and Wulf Wulfhekel<sup>1,6</sup>

<sup>1</sup>*Physikalisches Institut, Karlsruhe Institute of Technology, 76131 Karlsruhe, Germany*

<sup>2</sup>*Institute for Quantum Materials and Technologies,  
Karlsruhe Institute of Technology, 76131 Karlsruhe, Germany*

<sup>3</sup>*Universite de Lorraine, Institute Jean Lamour, France*

<sup>4</sup>*Department of Materials Science, Chiba University,  
1-33 Yayoi-cho, Inage-ku, Chiba 263-8522, Japan*

<sup>5</sup>*Molecular Chirality Research Centre, Chiba University,  
1-33 Yayoi-cho, Inage-ku, Chiba 263-8522, Japan*

<sup>6</sup>*Institute for Quantum Materials and Technologies,  
Karlsruhe Institute of Technology, 76344 Eggenstein-Leopoldshafen, Germany*

<sup>7</sup>*Institut für Theorie der Kondensierten Materie,  
Karlsruhe Institute of Technology, 76131 Karlsruhe, Germany*

(Dated: May 12, 2025)

## CONTENTS

|                                                                                |    |
|--------------------------------------------------------------------------------|----|
| I. Stacking fault tetrahedrons on Pb(111)                                      | 2  |
| II. Quantum well states on SFTs                                                | 3  |
| III. Intrinsic superconducting gaps of Pb(111)                                 | 3  |
| IV. Screw dislocations on Pb(111)                                              | 7  |
| V. Quasiparticle interferences by SFTs                                         | 7  |
| VI. Validity of the S&W model                                                  | 9  |
| VII. Influence of intra-band couplings in S&W model                            | 9  |
| VIII. Spatially resolved normal density of states for different Fermi surfaces | 11 |
| IX. SFT with enhanced DOS in triangle region                                   | 11 |
| References                                                                     | 13 |

## I. STACKING FAULT TETRAHEDRONS ON PB(111)

Stacking fault tetrahedrons (SFTs) are low-energy defects in face-centered cubic (fcc) crystals that have been extensively studied, e.g. in Au [1–6], Ag [7–10], Cu [11], and Al [12]. However, they are less reported in Pb(111) [13]. Figure S1(a) shows a topography with terraces and monolayer steps. On the terraces, there are many small Ar-induced vacancies and Ar bubbles buried beneath the surface. A screw dislocation can also be seen. In addition, there is a dark triangle with a lateral length about 30 nm on the surface [Fig. S1(a)] which is a stacking fault tetrahedrons on Pb(111). First, the step height on the surface above the SFT is approximately 1/3 of a monolayer [Fig. S1(b)] in agreement with the expected Burgers vector and similar results on SFTs reported by Wolf and Ibach [7]. Second, from the atomic resolution of the surface, we identify the edges of the triangle that follow the  $\langle 110 \rangle$  directions on the (111) surface [Fig. S1(c)], which are the directions of the expected

\* These authors contributed equally to this work.

† These authors contributed equally to this work.; Corresponding author: qili.li@kit.edu

stair-rod dislocations of the SFT [14, 15]. Due to crysallography, all SFTs in our sample have a similar shape and orientation. In fact, we observed more than 20 SFTs and the orientation of the triangle, i.e. the orientation of the SFT, is the same in all cases. The side lengths of the SFTs range from 20 to more than 100 nm. In contrast to normal conducting fcc metals, Pb allows to explore the influence of SFTs on superconductivity. Figure S1(d) shows the corresponding  $dI/dU$  map at  $\Delta_2^0$ , which shows an enhanced superconducting density of states outside the triangle similar to the SFTs shown in Fig. 1.

## II. QUANTUM WELL STATES ON SFTS

The quantum well states (QWSs) in Pb thin films on Si(111) are well known for the quantum size effect [16]. Moreover, QWSs also exist in Pb thin film on Cu(111) [17]. For single crystal Pb (111), QWSs are observed by STM atop subsurface vacancy clusters [18–20]. Unsurprisingly, we also observed QWSs on SFTs in Pb(111) as the involved stacking faults induce scattering for electrons in Pb(111). Similar electronically decoupling SFTs are also found in Ag(111) [9] and Au(111) [6] films. Figure S2(a) shows the topography of an SFT with side length about 20 nm. The  $dI/dU$  spectrum on the center of the stacking fault tetrahedron presents a series of peaks, i.e. QWSs [Fig. S2(b), magenta curve]. QWSs are absent outside the SFT [Fig. S2(b), blue curve]. Using the dispersion along  $\overline{\Gamma L}$  and the measured energy spacing of QWSs, the depth of the SFT can be estimated to be about 20 nm below the surface [21–23].

Figure S3 shows  $dI/dU$  maps for different energies, which correspond to peaks in Fig. S2(b). We observe two main characteristics: First, the QWSs exist only on the triangle (bright) and no states outside the triangle (dark). Second, the maps show uniform, high differential conductance for the energy larger than 980 meV. Between 980 meV and 360 meV, weak lateral confinements can be observed. Below 360 meV, the  $dI/dU$  intensity tends to be uniform again. This can be understood by the bandstructure of Pb [18, 19].

## III. INTRINSIC SUPERCONDUCTING GAPS OF Pb(111)

To determine the intrinsic superconducting gaps of Pb(111), we measured the scanning tunneling spectroscopy (STS) on defect-free area of Pb(111), where there is no influence from

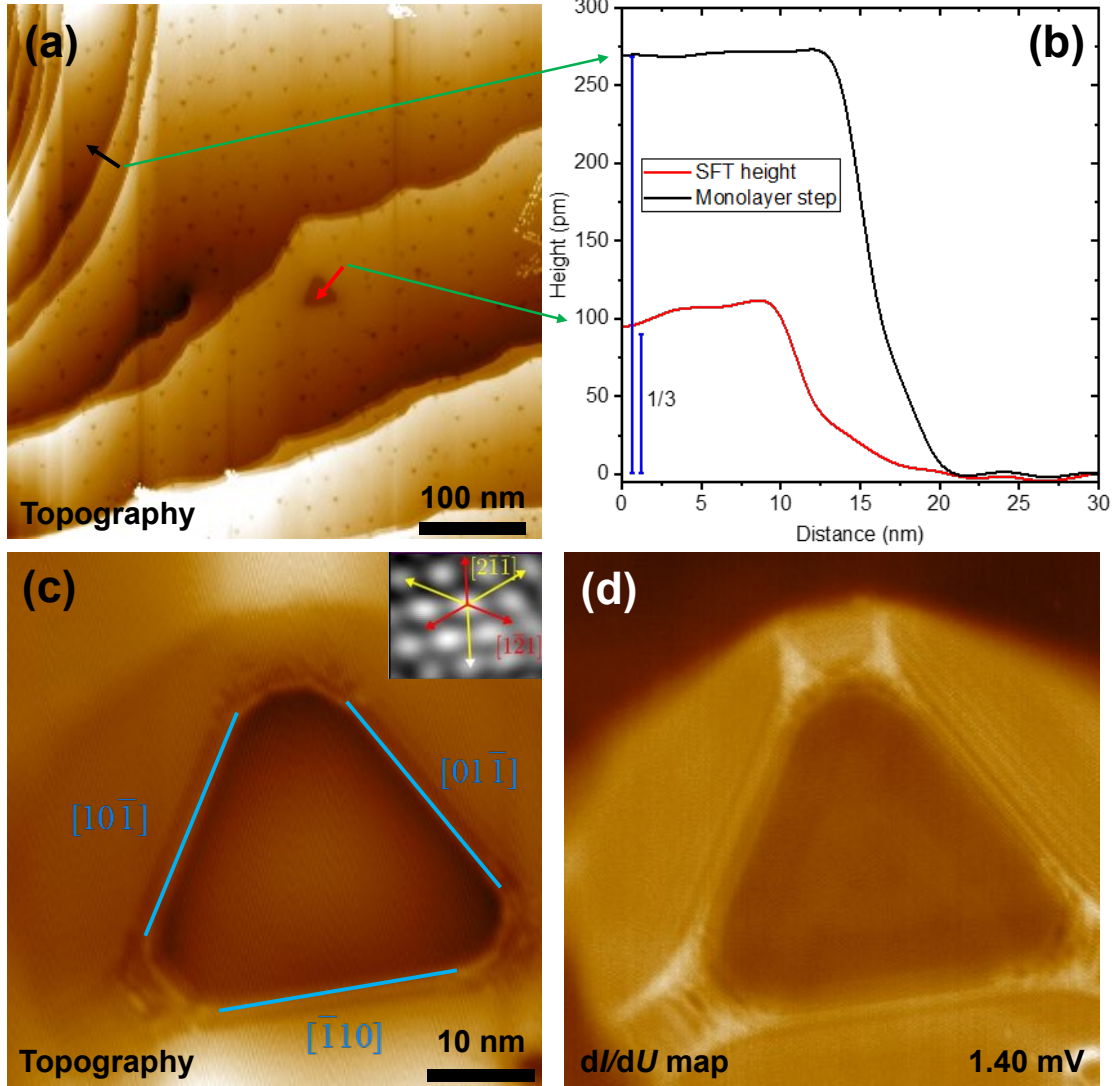

FIG. S1. Stacking fault tetrahedron on Pb(111) (SFT#4). (a) An SFT with a side length of  $\sim 30$  nm on the Pb(111) surface. The tip was stabilized at  $U = 100$  mV and  $I = 50$  pA. (b) The distance between the SFT and the surface is 95 pm, which is equal to  $1/3$  of the monolayer step height. Note that the next lower terrace is set to zero as reference. This is a fingerprint of an SFT on a (111) surface. (c) Zoom-in topography shows that the directions along which the edges of the triangle are oriented are  $\langle 110 \rangle$ , which is identified by the atomic resolution in the inset. The edges of the triangle are actually the stair rods to two intersected 111 surfaces. (d) The  $dI/dU$  map at the energy of  $\Delta_2^0$  shows the enhanced superconducting density of states outside the triangle. The tip was stabilized at  $U = 1.40$  mV and  $I = 100$  pA. The lock-in amplifier had modulation of  $50 \mu\text{V}$  and frequency of 3.751 kHz.

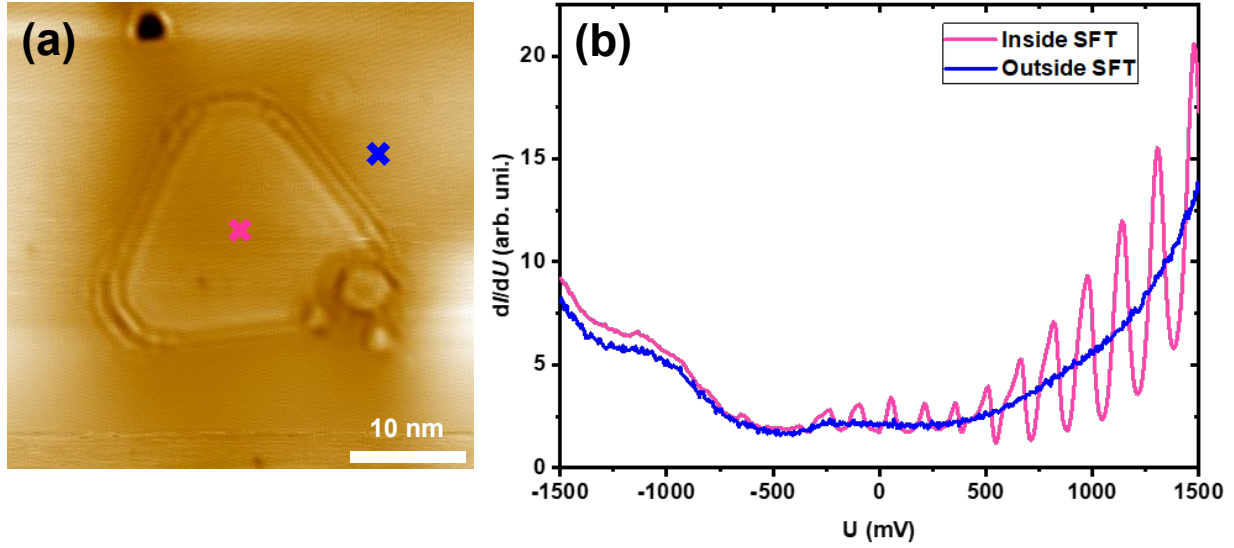

FIG. S2. Quantum well states on a stacking fault tetrahedron (SFT#2). (a) Topographic image of a subsurface SFT. (b)  $dI/dU$  spectra inside (magenta) and outside (blue) of SFT as marked by the magenta and blue crosses in (a), respectively. The tip was stabilized with sample bias  $U = 1.5$  V and tunneling current  $I = 1.0$  nA at a temperature of 46 mK. The lock-in modulation has an amplitude of 10 mV and a frequency of 3.352 kHz. The depth of this SFT is about 20 nm below the surface as determined from energy spacings of the quantum well states.

any defects in an area of  $30 \text{ nm} \times 30 \text{ nm}$ . Figure S4 shows the defect-free spectra, which were fitted by different models. Note that in the STS measurements, the tip was stabilized at  $U = 3$  mV and  $I = 1$  nA with modulation amplitude  $U_{mod} = 20 \text{ } \mu\text{V}$  and frequency 3.041 kHz.

Figure S4(a) shows the defect-free spectra fitted by Suhl-Matthias-Walker model [24] with BCS quasiparticle density of states (DOS) for each band (SMW-BCS). The temperature broadening is also incorporated into the SMW-BCS fitting by convolution with the first derivative of the Fermi-Dirac function here and after. Figure S4(b) shows the defect-free spectra fitted by Suhl-Matthias-Walker model [24] with Dynes formula for each band (SMW-Dynes). Figure S4(c) shows the Sung-Wong model [25] (S&W) fitting. These different fittings result in the same gaps within the error bar, i.e.  $\Delta_1^0 = 1.252 \pm 0.001$  meV and  $\Delta_2^0 = 1.400 \pm 0.001$  meV. The consistent gaps are obtained by superconducting tip measurements [26, 27]. However, the SMW-BCS does not capture the height of coherence

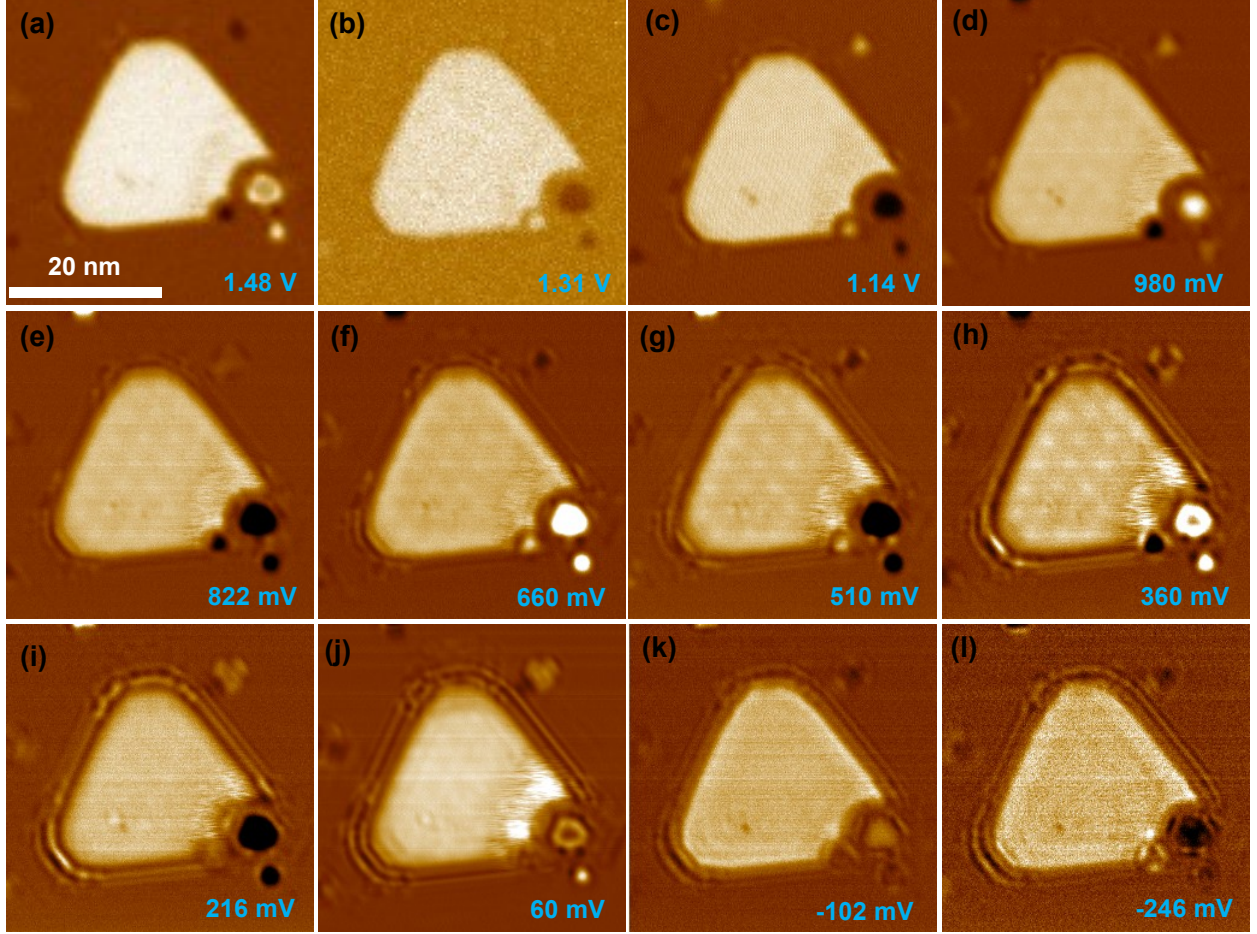

FIG. S3.  $dI/dU$  maps at various bias voltages displaying quantum well states between the SFT#2 and the surface. The maps show almost uniform high local density of states in the triangle region and low local density of states outside the triangle.

peak  $\Delta_2^0$  Figure S4(a). When using SMW-Dynes model to fit, both gaps can be well fitted with very small intra-band couplings  $\Gamma_1 = 0$  and  $\Gamma_2 = 27 \mu\text{eV}$ . As expected, the S&W model fitting obtained an almost zero inter-band coupling  $\Gamma_{21}$ . The other fitting parameters are listed in Table I. We point out that the electronic temperature in our measurements at 45 mK is about 82 mK [28]. The S&W model fits better than SMW-Dynes model in the sense of electronic temperature.

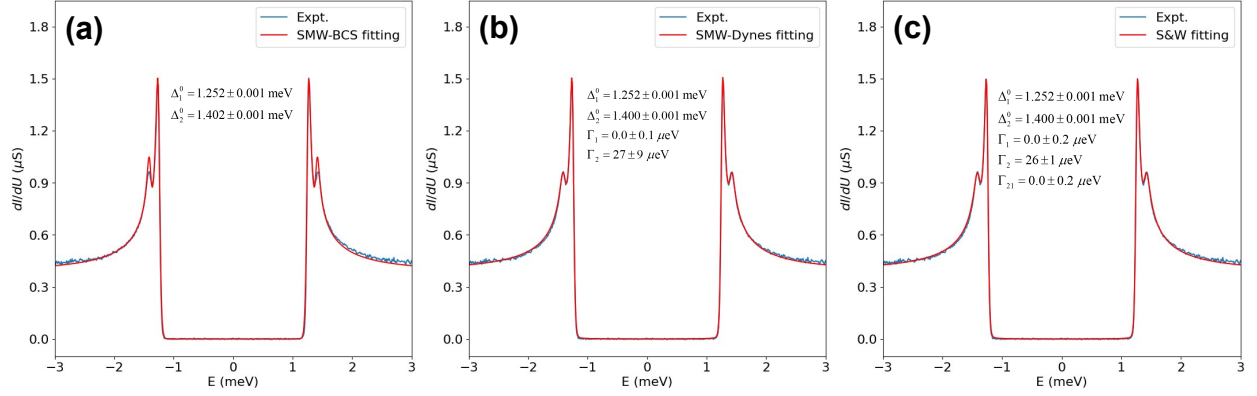

FIG. S4. Determining the intrinsic gaps of Pb(111) from defect-free spectra. (a) Fitted by SMW-BCS model. (b) Fitted by SMW-Dynes model. (c) Fitted by S&W model.

TABLE I. Other fitted parameters for defect-free spectra.

| Models    | $\sigma_1^0 (\mu S)$ | $\sigma_2^0 (\mu S)$ | $T$ (mK)    |
|-----------|----------------------|----------------------|-------------|
| SMW-BCS   | $0.306 \pm 0.001$    | $0.075 \pm 0.001$    | $193 \pm 2$ |
| SMW-Dynes | $0.288 \pm 0.001$    | $0.097 \pm 0.001$    | $174 \pm 1$ |
| S&W       | $0.288 \pm 0.001$    | $0.097 \pm 0.001$    | $139 \pm 1$ |

#### IV. SCREW DISLOCATIONS ON PB(111)

Screw dislocations are another common defect in fcc crystals [7, 29, 30]. Figure S5(a) shows a screw dislocation on the surface marked by the arrow. We also measured the  $dI/dU$  map at the energy of  $\Delta_2^0$  (1.40 mV) around this screw dislocation, as shown in Fig. S5(b). However, we did not observe any enhanced superconducting coherence peak compared with that in the defect-free area. It indicates that screw dislocations have no influence on superconducting gaps in Pb(111).

#### V. QUASIPARTICLE INTERFERENCES BY SFTS

Quasiparticle interference (QPI) around Fermi energy can be seen in the triangles in Figs. 1 and 3. We point out that these QPIs are not due to superconducting states, as they do not change when superconductivity is suppressed by a magnetic field [Fig. 3(c)]. Therefore, these patterns arise from the scattering of normal electron states around the

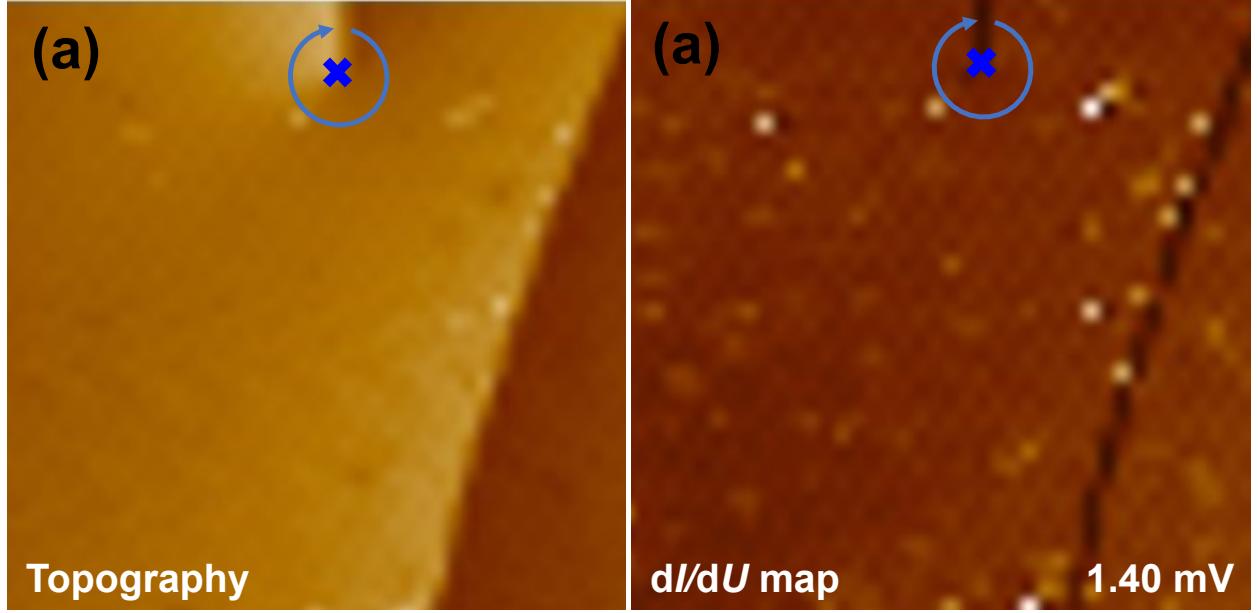

FIG. S5. Screw dislocation on Pb(111). (a) Topography of a screw dislocation near a monolayer step edge. (b) The  $dI/dU$  map at the energy of  $\Delta_2^0$  (1.40 mV).

Fermi energy. To quantify QPIs, we Fourier transformed the  $dI/dU$  maps [Fig. S6(a,d)]. Figures S6(b,e) show the reciprocal maps for QPI inside the triangles. The wave number is about  $0.13 \times (2\pi/a)$  in the large SFT [Fig. S6(a)], while it is about  $0.2 \times (2\pi/a)$  in the small SFT [Fig. S6(d)].

To determine the QPI scattering vector, we used DFT to calculate the projected DOS for open [Fig. S6(c)] and compact [Fig. S6(f)] Fermi surfaces. The sum of projected DOS of two Fermi surfaces is shown in Fig. S6(g). Note that these results were obtained by first calculating band energies via DFT on a very dense  $100 \times 100 \times 100$   $k$  mesh. The energies were then linearly interpolated to perform the projection using 800 points along  $k_z$  and a Gaussian broadening of 0.1 eV. The observed scattering vectors (length and direction) can be found in the projected DOS to connect flat parts of the open and compact Fermi surfaces, as indicated by the yellow lines. In the large SFT [Fig. S6(a)], the LDOS for the compact Fermi surface is almost zero, so only the intra-band scattering for open Fermi surface is seen, which corresponds to the short yellow line in Fig. S6(c). However, for the small SFT [Fig. S6(d)], the LDOS for compact and open Fermi surfaces are comparable, so the inter-band scattering between compact and open Fermi surfaces is observed, which corresponds to the long yellow line in Fig. S6(g). These results are consistent with our S&W fittings

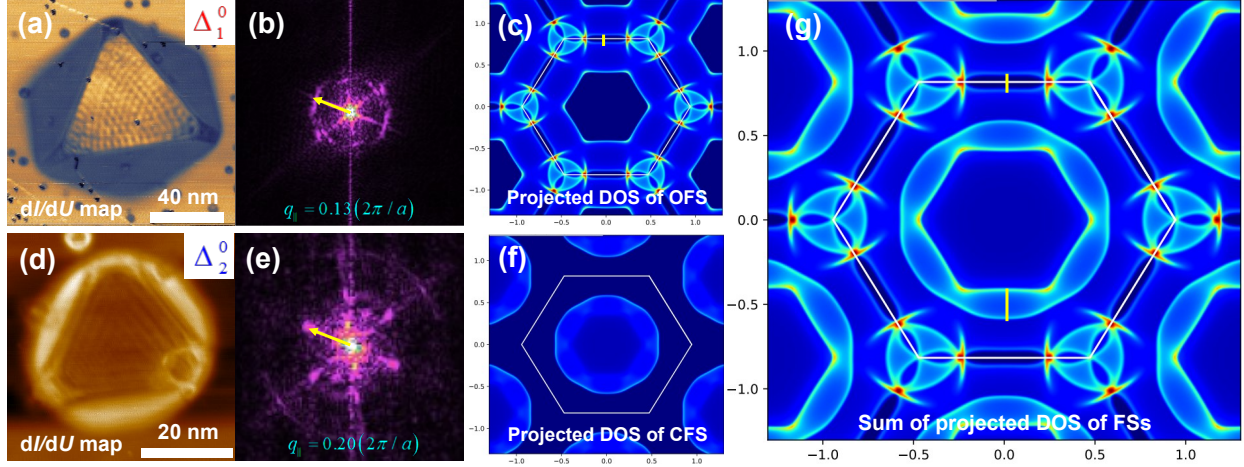

FIG. S6. Quasiparticle interferences by SFTs (SFT#1 and #2). (a) The  $dI/dU$  map at  $\Delta_1^0$  (SFT#1). (b) Fourier transform of (a). (c) The calculated projected DOS of open Fermi surface (OFS) by DFT. (d) The  $dI/dU$  map at  $\Delta_2^0$  (SFT#2). (e) Fourier transform of (d). (f) The calculated projected DOS of compact Fermi surface (CFS) by DFT. (g) The sum of projected DOS of two Fermi surfaces. The yellow lines are the nesting vectors of the QPIs.

that strong intra- and inter-band scatterings exist in the triangle region.

## VI. VALIDITY OF THE S&W MODEL

We compared the fitting for spectra in hexagon region of SFT by SMW-Dynes and S&W models Fig. S7. The Dynes fit does not fully reproduce the experimental data. First of all, the gap edge cannot be well fitted (see Fig. S7(a)). Secondly, the smooth transition from small coherence peak to the large coherence cannot be captured. Thirdly,  $\Delta_1$  increases compared with defect-free fitting, while  $\Delta_2$  remains the same within error bar. When using the S&W model to fit, both the gap edge and smooth transition are well fitted [Fig. S7(b)]. More importantly, we can easily understand that the increased  $\Delta_1$  is actually from inter-band coupling, which shifts the  $\Delta_1$  towards  $\Delta_2$  a bit.

## VII. INFLUENCE OF INTRA-BAND COUPLINGS IN S&W MODEL

The intra-band couplings can also modify the quasiparticle spectroscopy of superconducting gaps. Figure S8 demonstrates the influence of intra-band couplings. We can see that the

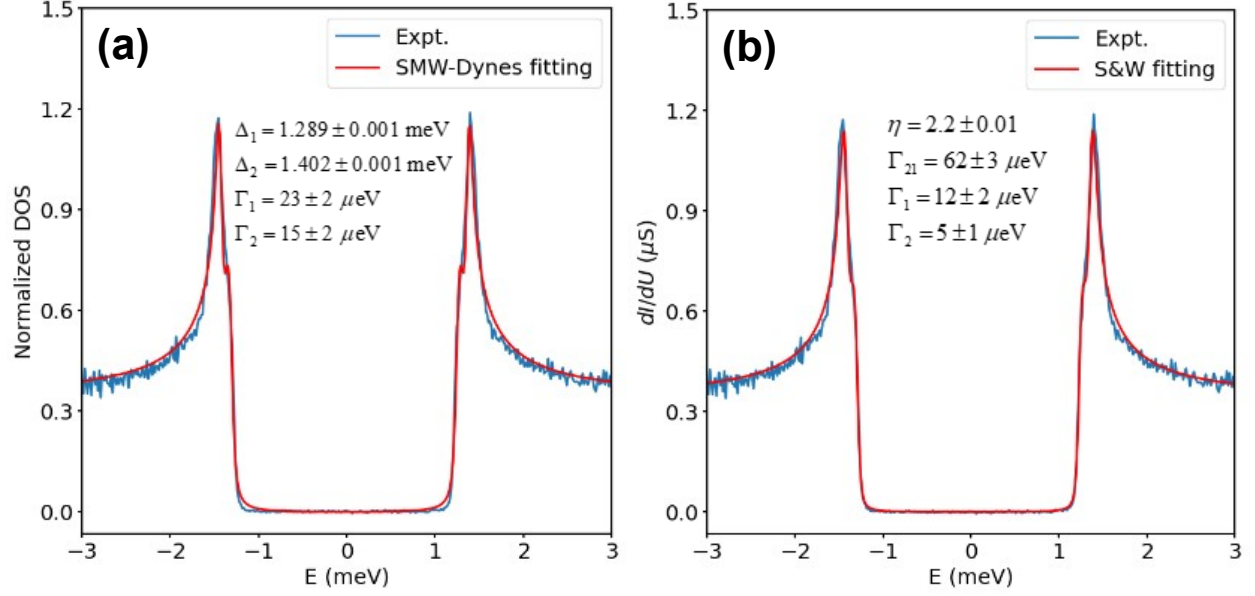

FIG. S7. Validity of the S&W model. (a) The spectra in hexagon region of SFT#1 were fitted by SMW-Dynes model, the other fitted parameters are  $\sigma_1 = 0.184 \pm 007$   $\mu$ S and  $\sigma_2 = 0.163 \pm 007$   $\mu$ S. (b) The same spectra fitted by S&W model with  $\sigma_1 = 0.136 \pm 003$   $\mu$ S. The effective temperature 139 mK obtained from defect-free spectra was fixed in the fittings.

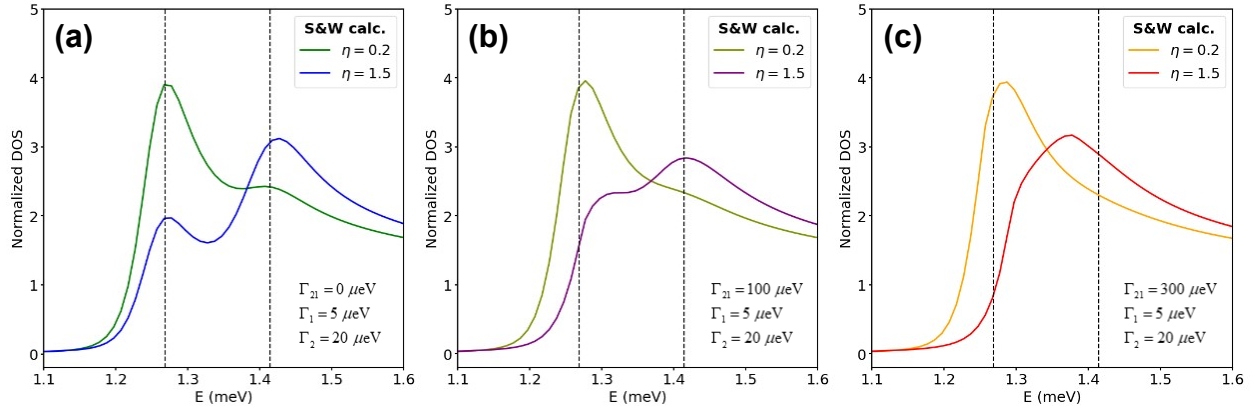

FIG. S8. Influence of intra-band couplings. The broadening effect of intra-band couplings decreases the intensities of coherence peaks and rounds the gap edges.

intensities of coherence peaks decrease and the gap edges are not sharp any more compared with Figs. 2(a)-(c).

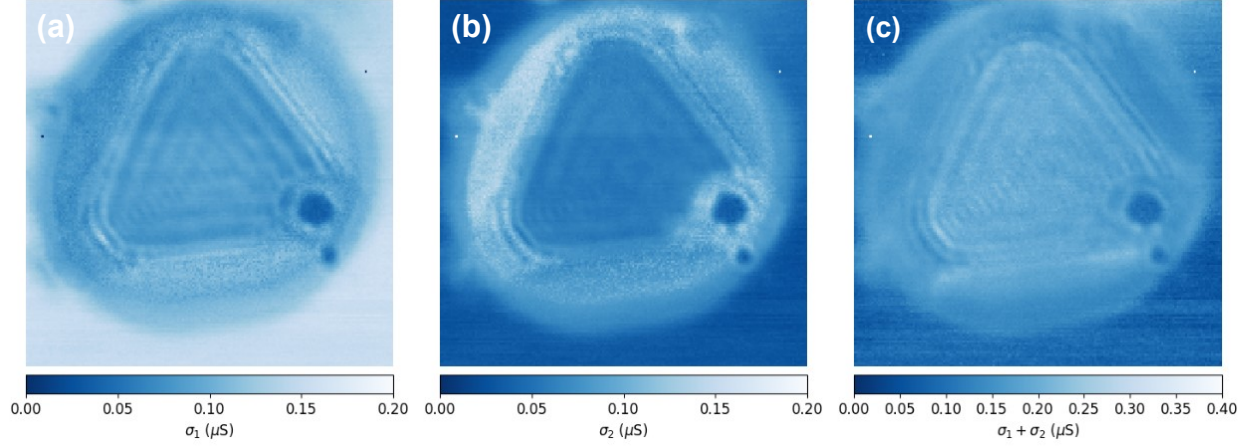

FIG. S9. Spatially resolved normal density of states for different Fermi surfaces (SFT#2). (a) The differential conductance  $\sigma_1$  for the open Fermi surface. (b) The differential conductance  $\sigma_2$  for the close Fermi surface. (c) Total differential conductance  $\sigma_1 + \sigma_2$ .

### VIII. SPATIALLY RESOLVED NORMAL DENSITY OF STATES FOR DIFFERENT FERMI SURFACES

With S&W model [25] fitting, we can also obtain information about the normal states of these two different Fermi surfaces. Figure S9(a) shows the differential conductance  $\sigma_1$  at the Fermi energy for  $\Delta_1$ , which corresponds to the open Fermi surface [inset in Fig.1 (c)]. We can see the interference inside the triangle and the reduced intensity in region II, which is similar to the  $dI/dU$  map in Fig. 3(a). The calculated differential conductance  $\sigma_2$  at Fermi energy is shown in Fig. S9(b). The corresponding Fermi surface is the compact one shown as inset in Fig.1(d). The total differential conductance, i.e. the sum of  $\sigma_1 + \sigma_2$  [Fig. S9(c)].

### IX. SFT WITH ENHANCED DOS IN TRIANGLE REGION

We show another SFT with side length about 16 nm. In this SFT, we still see a similar contrast in hexagon region for  $dI/dU$  maps at energy  $\Delta_1^0$  Fig. S10(a) and  $\Delta_2^0$  Fig. S10(b). However, this SFT has an enhanced DOS in the triangle region Fig. S10(c), which is different from the SFT in Fig. 3 in the main text. This is due to its different depth causing an enhanced LDOS by the QWS. The obtained intra- and inter-band couplings are shown in Fig. S11, which have patterns similar with Fig. 4. The fitted differential conductance  $\sigma_i$  is

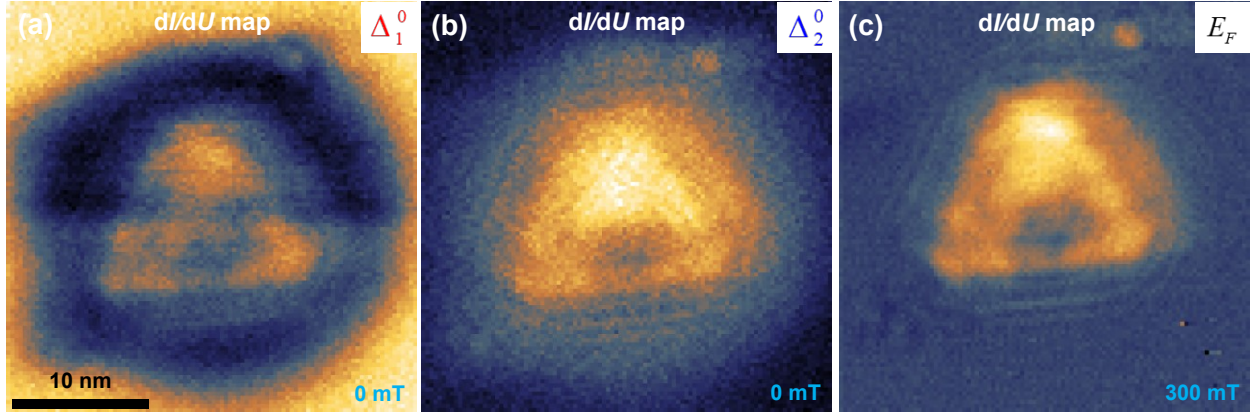

FIG. S10. SFT#3 with enhanced DOS in triangle region. (a)  $dI/dU$  map at energy  $\Delta_1^0$ . (b)  $dI/dU$  map at energy  $\Delta_2^0$ . (c)  $dI/dU$  map at energy  $E_F$  with magnetic field 300 mT.

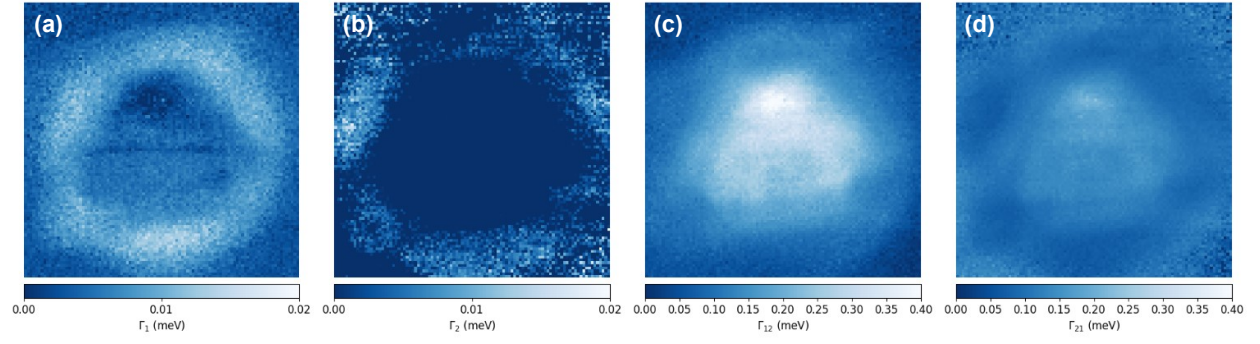

FIG. S11. The spatially resolved intra- and inter-band couplings for SFT#3 with enhanced DOS in triangle region. (a) The intra-band coupling  $\Gamma_1$ . (b) The intra-band coupling  $\Gamma_2$ . (c) The inter-band coupling  $\Gamma_{12}$ . (d) The inter-band coupling  $\Gamma_{21}$ .

shown in Fig. S12.

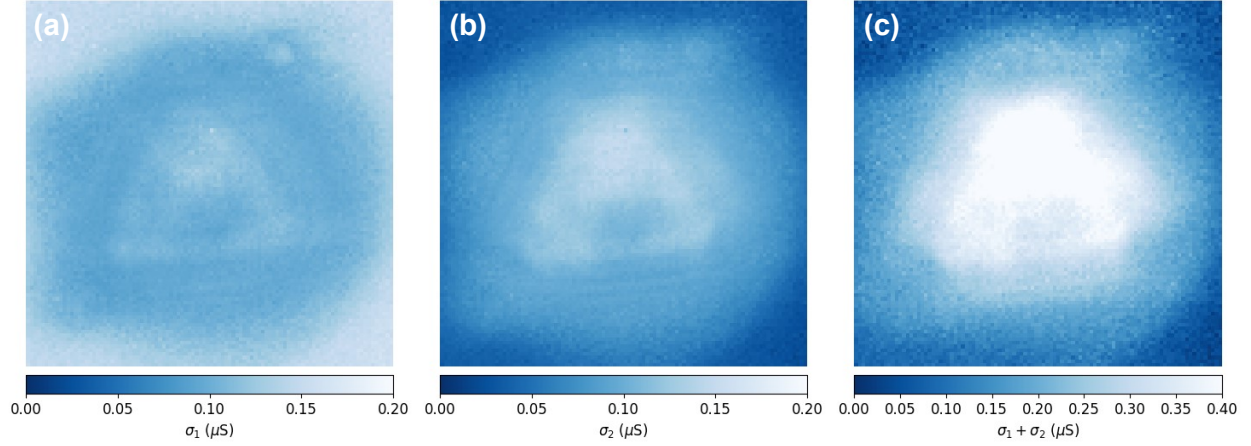

FIG. S12. Spatially resolved normal density of states of different Fermi surfaces for SFT#3 with enhanced DOS in triangle region. (a) The differential conductance  $\sigma_1$  for the open Fermi surface. (b) The differential conductance  $\sigma_2$  for the close Fermi surface. (c) Total differential conductance  $\sigma_1 + \sigma_2$ .

- 
- [1] J. Silcox and P. B. Hirsch, *Philos. Mag.* **4**, 72 (1959).
  - [2] R. M. J. Cotterill, *Philos. Mag.* **6**, 1351 (1961).
  - [3] M. J. Yokota and J. Washburn, *Philos. Mag.* **16**, 459 (1967).
  - [4] Y. Matsukawa, Y. N. Osetsky, R. E. Stoller, and S. J. Zinkle, *Philos. Mag.* **88**, 581 (2008).
  - [5] J. Wei Wang, S. Narayanan, J. Yu Huang, Z. Zhang, T. Zhu, and S. X. Mao, *Nat. Commun.* **4**, 2340 (2013).
  - [6] K. Schouteden, B. Amin-Ahmadi, Z. Li, D. Muzychenko, D. Schryvers, and C. Van Haesendonck, *Nat. Commun.* **7**, 14001 (2016).
  - [7] J. F. Wolf and H. Ibach, *Appl. Phys. A* **52**, 218 (1991).
  - [8] G. J. Hardy and M. L. Jenkins, *Philos. Mag.* **52**, L19 (2006).
  - [9] K. Schouteden and C. Van Haesendonck, *Phys. Rev. Lett.* **108**, 076806 (2012).
  - [10] K. Y. Yu, D. Bufford, C. Sun, Y. Liu, H. Wang, M. A. Kirk, M. Li, and X. Zhang, *Nat. Commun.* **4**, 1377 (2013).
  - [11] R. Schäublin, Z. Yao, N. Baluc, and M. Victoria, *Philos. Mag.* **85**, 769 (2005).

- [12] Q. F. Guan, L. Pan, H. Zou, A. M. Wu, S. Z. Hao, Q. Y. Zhang, C. Dong, and G. T. Zou, J. Mater. Sci. **39**, 6349 (2004).
- [13] F. Bonsignori, V. Bortolani, and G. Velo, Nuovo Cimento B **57**, 194 (1968).
- [14] M. Ohmori, H. Hirayama, and K. Takayanagi, Phys. Rev. B **59**, 5612 (1999).
- [15] Y. N. Osetsky, D. Rodney, and D. J. Bacon, Philos. Mag. **86**, 2295 (2006).
- [16] Y. Guo, Y.-F. Zhang, X.-Y. Bao, T.-Z. Han, Z. Tang, L.-X. Zhang, W.-G. Zhu, E. G. Wang, Q. Niu, Z. Q. Qiu, J.-F. Jia, Z.-X. Zhao, and Q.-K. Xue, Science **306**, 1915 (2004).
- [17] M. Schackert, T. Märkl, J. Jandke, M. Hölzer, S. Ostanin, E. K. U. Gross, A. Ernst, and W. Wulfhekel, Phys. Rev. Lett. **114**, 047002 (2015).
- [18] M. Müller, N. Néel, S. Crampin, and J. Kröger, Phys. Rev. Lett. **117**, 136803 (2016).
- [19] M. Müller, N. Néel, S. Crampin, and J. Kröger, Phys. Rev. B **96**, 205426 (2017).
- [20] S. Y. Song and J. Seo, Sci. Rep. **7**, 12177 (2017).
- [21] O. Kurnosikov, O. A. O. Adam, H. J. M. Swagten, W. J. M. de Jonge, and B. Koopmans, Phys. Rev. B **77**, 125429 (2008).
- [22] O. Kurnosikov, J. H. Nietsch, M. Sicot, H. J. M. Swagten, and B. Koopmans, Phys. Rev. Lett. **102**, 066101 (2009).
- [23] O. Kurnosikov, H. J. M. Swagten, and B. Koopmans, Phys. Rev. Lett. **106**, 196803 (2011).
- [24] H. Suhl, B. T. Matthias, and L. R. Walker, Phys. Rev. Lett. **3**, 552 (1959).
- [25] C. C. Sung and V. K. Wong, J. Phys. Chem. Solids **28**, 1933 (1967).
- [26] M. Ruby, B. W. Heinrich, J. I. Pascual, and K. J. Franke, Phys. Rev. Lett. **114**, 157001 (2015).
- [27] M. Uhl, P. Kot, R. Drost, H. Huang, J. Ankerhold, J. C. Cuevas, and C. R. Ast, Phys. Rev. Res. **6**, 043233 (2024).
- [28] T. Balashov, M. Meyer, and W. Wulfhekel, Rev. Sci. Instrum. **89**, 113707 (2018).
- [29] J. Engbæk, J. Schiøtz, B. Dahl-Madsen, and S. Horch, Phys. Rev. B **74**, 195434 (2006).
- [30] A. Y. Aladyshkin, A. S. Aladyshkina, and S. I. Bozhko, J. Phys. Chem. C **125**, 26814 (2021).
